# Supplementary material for: The Satisfiability Threshold for K-XOR Games
Source: arXiv:2505.01628 ancillary file (2025-05-02)
Supplement: Supplementary file 1 [file critical-sets-K-XOR-GAME-v1-2025-May-02.nb.pdf]

# Mathematica Notebook: Interval Arithmetic Supporting “The Satisfiability Threshold for K-XOR Games” v1 (2025 May 02)

This notebook accompanies the paper “The Satisfiability Threshold for K-XOR Games” by Jared A. Hughes and J. William Helton.

Firstly, “General-Purpose Commands” defines some commands for helping interval arithmetic and checking if a function is positive on a rectangle.

Then “Helper Functions for K-XORGAME” defines functions such as Q and H that are specific to evaluating the  $J_K$  function for K-XORGAME.

Finally, “Interval arithmetic towards proving  $J_K < -\epsilon$  for  $2 < c < K$ .” uses interval arithmetic to verify various claims that are used in the paper to eventually show  $J_K < -\epsilon$  on a large rectangle.

## General-Purpose Commands

---

Commands: Proving a function is positive on a 1D or 2D rectangle using gridding.

We use “gridding” to denote the process of applying interval arithmetic on a set of smaller rectangles covering a larger rectangle.

## Command: uniform grid on 1D interval

```
In[ ]:= (*
Split up the interval intλ uniformly into nλ sub-intervals,
and return all sub-intervals where the `keep` function holds true.
*)
UniformGrid1D[keep_, intλ_Interval, nλ_Integer] :=
#[] & /@ Select[Not[False === #[]] &]@ParallelTable[With[{
λ = Min@intλ + (Max@intλ - Min@intλ) *  $\frac{\text{Interval}[\{i\lambda, i\lambda + 1\}]}{n\lambda}$ 
}, {λ, keep[λ]}, {iλ, 0, nλ - 1}]

(*
Split up the interval intλ uniformly into nλ sub-intervals,
and return all sub-intervals where the function `fn` is provably positive.
*)
UniformGridPositive1D[fn_, intλ_Interval, nλ_Integer] :=
UniformGrid1D[λ ↦ Not[True === (fn[λ] > 0)], intλ, nλ]
```

```
In[ ]:= UniformGridPositive1D[λ ↦ λ, Interval[{-1.0, 1.0}], 5]
```

```
Out[ ]:= {Interval[{-1., -0.6}], Interval[{-0.6, -0.2}], Interval[{-0.2, 0.2}]}
```

```
In[ ]:= UniformGridPositive1DwithStatement[fn_, intλ_Interval, nλ_Integer] := Module[{x},
x = Timing@UniformGridPositive1D[fn, intλ, nλ];
problems = x[];
Print["Problems: ", Length@problems, " in ", x[], "s."];
If[Length@problems > 0,
Print["First problem: ", problems[],
Print["Success on ", intλ]
];
]
```

## Examples of UniformGridPositive1DwithStatement[].

```
In[ ]:= UniformGridPositive1DwithStatement[λ ↦ λ, Interval[{-1.0, 1.0}], 5]
```

```
Problems: 3 in 0.004745s.
```

```
First problem: Interval[{-1., -0.6}]
```

```
In[ ]:= UniformGridPositive1DwithStatement[λ ↦ λ + 1.1, Interval[{-1.0, 1.0}], 5]
```

Problems: 0 in 0.006691s.

Success on Interval[{-1., 1.}]

## Command: uniform grid on 2D rectangle

```
In[ ]:= (*
Split up the rectangle intλ × intα uniformly into nλ × nα sub-rectangles,
and return all sub-rectangles where the `keep` function holds true
*)
UniformGrid2D[keep_, intλ_Interval, nλ_Integer, intα_Interval, nα_Integer] :=
#[[1]]&@Select[Not[False===#[[2]]]&]@Flatten[ParallelTable[With[{
λ=Min@intλ+(Max@intλ-Min@intλ)* $\frac{\text{Interval}[\{i\lambda, i\lambda+1\}]}{n\lambda}$ ,
α=Min@intα+(Max@intα-Min@intα)* $\frac{\text{Interval}[\{i\alpha, i\alpha+1\}]}{n\alpha}$ 
}], {{λ, α}, keep[λ, α]}, {iλ, 0, nλ-1}, {iα, 0, nα-1}], 1]

(* Split up the rectangle intλ × intα uniformly into nλ × nα sub-rectangles,
and return all sub-rectangles where the function `fn` is provable positive *)
UniformGridPositive2D[fn_, intλ_Interval, nλ_Integer, intα_Interval, nα_Integer]:=
UniformGrid2D[{λ, α}↦Not[True===(fn[λ, α]>0)], intλ, nλ, intα, nα]

In[ ]:= UniformGridPositive2D[{λ, α}↦λ*α, Interval[{-1.0, 1.0}], 3, Interval[{-1.0, 1.0}], 3]

Out[ ]:= {{Interval[{-1., -0.333333}], Interval[{-0.333333, 0.333333}]},
{Interval[{-1., -0.333333}], Interval[{0.333333, 1.}]},
{Interval[{-0.333333, 0.333333}], Interval[{-1., -0.333333}]},
{Interval[{-0.333333, 0.333333}], Interval[{-0.333333, 0.333333}]},
{Interval[{-0.333333, 0.333333}], Interval[{0.333333, 1.}]},
{Interval[{0.333333, 1.}], Interval[{-1., -0.333333}]},
{Interval[{0.333333, 1.}], Interval[{-0.333333, 0.333333}]}}
```

```

In[ ]:= (*
Split up the rectangle  $\text{int}\alpha \times \text{int}\lambda$  uniformly into  $n\alpha \times n\lambda$  sub-rectangles,
with the goal to prove the `fn` is positive on each sub-rectangle.
  Displays (in red) the sub-rectangles on which it fails to prove `fn` is positive,
  along with the count of failing sub-rectangles.
*)
UniformGridPositive2DwithPicture[fn_, int $\alpha$ _Interval,
  n $\alpha$ _Integer, int $\lambda$ _Interval, n $\lambda$ _Integer] := Module[{x, plot, gridLines},
  x = Timing@UniformGridPositive2D[fn, int $\alpha$ , n $\alpha$ , int $\lambda$ , n $\lambda$ ];
  problems = x[[2]];
  Print["Problems: ", Length@problems, " in ", x[[1]], "s."];
  If[Length@problems > 0,
    Print["First problem: ", problems[[1]],
      Print["Success on ", Rectangle[Min/@{int $\alpha$ , int $\lambda$ }, Max/@{int $\alpha$ , int $\lambda$ }}]
  ];
  gridLines = ListPlot[{}, AxesLabel  $\rightarrow$  { $\alpha$ ,  $\lambda$ },
    PlotRange  $\rightarrow$  {{Min@int $\alpha$ , Max@int $\alpha$ }, {Min@int $\lambda$ , Max@int $\lambda$ }}];
  Show[
    gridLines,
    Graphics[{Darker@Green, Rectangle[Min/@{int $\alpha$ , int $\lambda$ }, Max/@{int $\alpha$ , int $\lambda$ }}],
    Graphics[{Red, (pair  $\mapsto$  Rectangle[Min/@pair, Max/@pair])/@problems}]
  ]
]

```

## Examples of UniformGridPositive2DwithPicture[ ].

```

In[ ]:= (* Just an example: the green is all rectangles where we can prove  $\alpha + \lambda > 0$ . *)
UniformGridPositive2DwithPicture[{ $\alpha$ ,  $\lambda$ }  $\mapsto$   $\alpha + \lambda$ ,
  Interval[{-1.0, 1.0}], 5, Interval[{-1.0, 1.0}], 5]

```

Problems: 19 in 0.007221s.

First problem: {Interval[{-1., -0.6}], Interval[{-1., -0.6}]}

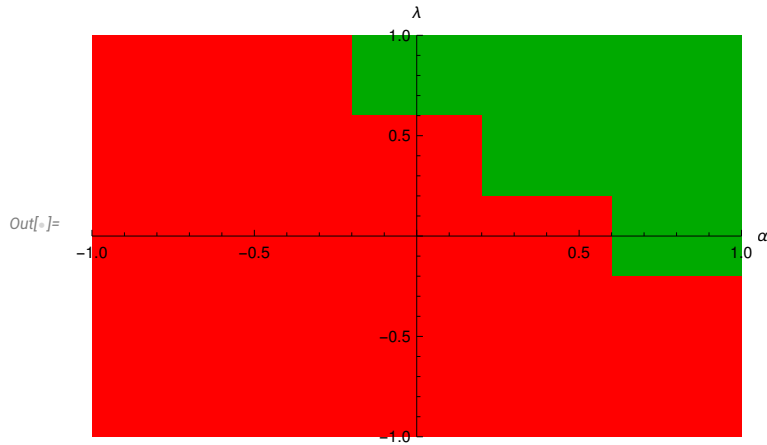

In[ ]:= (\* Another example: green is all rectangles where we can prove  $\alpha + \lambda + 2.1 > 0$ ,  
which is everywhere since  $\alpha \geq -1$  and  $\lambda \geq -1$ . \*)  
UniformGridPositive2DwithPicture[{ $\alpha$ ,  $\lambda$ }  $\mapsto$   $\alpha + \lambda + 2.1$ ,  
Interval[{-1.0, 1.0}], 5, Interval[{-1.0, 1.0}], 5]

Problems: 0 in 0.008058s.

Success on Rectangle[{-1., -1.}, {1., 1.}]

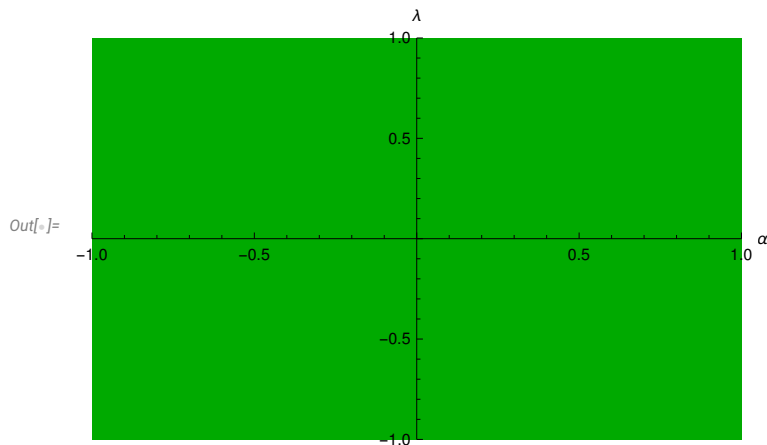

## General Interval Arithmetic Commands

```
In[ ]:= pointInterval[r_Real] := Interval[r]
pointInterval[r_Integer] := Interval[r]
pI = pointInterval;
```

```
In[ ]:= ParallelEvaluate[Off[Power::infy]]
```

Out[ ]:= {Null, Null, Null, Null}

```

In[ ]:= (* General::munfl is a message that displays when a floating
        point calculation underflows. This is a slight loss of precision,
        but it still produces valid intervals if given valid intervals input. (assuming) *)
        AllowUnderflow[e_] := Quiet[e, {General::munfl}]
        Off[General::munfl]
        SetAttributes[AllowUnderflow, {HoldAll}]
        AllowUnderflow[1.2 * 10^-308 * 0.0005]

```

```

Out[ ]:= 6. * 10^-312

```

Throughout the interval arithmetic definitions, we use helpers to keep the intervals narrow:

- `monotoneFuncInterval` assumes that the given function is increasing everywhere (or decreasing everywhere), so it can just be evaluated at the endpoints.
- `bimonotoneFuncInterval` assumes there is some parameter  $v$  such that the function  $f(z)$  is increasing for  $z < v$  and decreasing for  $z > v$  (or vice versa). Then only the endpoints need to be evaluated, except when the interval of  $z$  contains  $v$ , at which point  $f(v)$  needs to be evaluated as well.

```

In[ ]:= (* Take f on the values v, then find the smallest interval containing them all. *)
        intervalContainingPoints[a_] := Interval[{Min @@ (Min /@ a), Max @@ (Max /@ a)}]
        monotoneFuncIntervalPoints[f_, v_] := intervalContainingPoints[f /@ Interval /@ v]

        (* Assume f is either increasing everywhere or decreasing everywhere. *)
        monotoneFuncInterval[f_, z_Interval] :=
            AllowUnderflow@monotoneFuncIntervalPoints[f, {Min@z, Max@z}]

        (* Assume (weaker condition than convex): f is increasing for z <
            v and decreasing for z > v. (or resp. decreasing and increasing) *)
        bimonotoneFuncInterval[f_, z_Interval, v_] := AllowUnderflow@With[{m = Min[z], M = Max[z]},
            If[m < v && v < M, monotoneFuncIntervalPoints[f, {v, m, M}],
            monotoneFuncIntervalPoints[f, {m, M}]]]

```

## Multiply intervals (treating 0 correctly)

We work under the assumption that an exact “0” is an exact “0”, so multiplying it by any floating point is still an exact “0”. This differs from the default Mathematica interval behavior, where multiplying a floating point interval by an exact “0” gives a interval strictly containing floating point “0.0”.

```

In[ ]:= 0 * Interval[{0.0, 0.0}]
Out[ ]:= Interval[{-2.22507 * 10^-308, 2.22507 * 10^-308}]

```

```
In[ ]:= Clear[multiplyByZero]
multiplyByZero[b_Integer | b_Real | b_Rational] := 0
multiplyByZero[b_] := If[RealValuedNumericQ[b], 0, multiplyByZeroIndeterminate[b]]
```

```
In[ ]:= zeroOut[b_Interval] := multiplyByZero[Min@b] + multiplyByZero[Max@b]
```

```
In[ ]:= Clear[multiplyInterval]
multiply[a_, b_] := a * b
multiplyInterval[a_Interval, b_Interval] := If[Min@a === 0,
  If[Max@a === 0,
    Interval[zeroOut[b]],
    intervalContainingPoints[{zeroOut[b], Max@a * Min@b, Max@a * Max@b}]
  ],
  If[Max@a === 0,
    intervalContainingPoints[{zeroOut[b], Min@a * Min@b, Min@a * Max@b}],
    a * b
  ]
]
(* interval and non-interval*)
multiplyInterval[a_Interval, b_Real | b_Rational | b_Integer] :=
  multiplyInterval[a, Interval@b]
multiplyInterval[b_Real | b_Rational | b_Integer, a_Interval] :=
  multiplyInterval[Interval@b, a]
(* non-intervals and non-interval *)
multiplyInterval[a_Real | a_Rational | a_Integer,
  b_Real | b_Rational | b_Integer] := Interval[a * b];
multiplyInterval[a_, b_Interval] := a * b;
SetAttributes[multiplyInterval, Orderless];
multiplySymb = Inactive[multiply];
```

## Examples and testing

```

In[ ]:= multiplyByZero[7]
        multiplyByZero[2.0]
        multiplyByZero[2 / 3]
        multiplyByZero[Log[2]]
        multiplyByZero[Infinity]
        multiplyByZero[Indeterminate]
        multiplyByZero[unknownFunction]

Out[ ]:= 0

Out[ ]:= 0

Out[ ]:= 0

Out[ ]:= 0

Out[ ]:= multiplyByZeroIndeterminate[∞]

Out[ ]:= multiplyByZeroIndeterminate[Indeterminate]

Out[ ]:= multiplyByZeroIndeterminate[unknownFunction]

In[ ]:= multiplyInterval[Interval[{2, 5}], Interval[{2, 3}]]
        multiplyInterval[pI@0, Interval[{2, 3}]]
        multiplyInterval[0, Interval[{2, 3}]]
        multiplyInterval[0, Interval[{2.0, 3.0}]]
        multiplyInterval[Interval[{0, 3}], Interval[{2, 3}]]
        multiplyInterval[Interval[{-3, 0}], Interval[{2, 3}]]
        multiplyInterval[Interval[{0, 3}], Interval[{-2, 3}]]
        multiplyInterval[Interval[{-3, 0}], Interval[{-2, 3}]]
        multiplyInterval[x, Interval[{2, 3}]]

Out[ ]:= Interval[{4, 15}]

Out[ ]:= Interval[{0, 0}]

Out[ ]:= Interval[{0, 0}]

Out[ ]:= Interval[{0, 0}]

Out[ ]:= Interval[{0, 9}]

Out[ ]:= Interval[{-9, 0}]

Out[ ]:= Interval[{-6, 9}]

Out[ ]:= Interval[{-9, 6}]

Out[ ]:= x Interval[{2, 3}]

```

# Helper Functions for K-XORGAME



The sections below have the following conventions, where “function” stands for any of the functions considered below -- Q, expProd, nxLog, etc.:

function[z\_]:=symbolic definition

functionSymb = Inactive[function]

functionContinuous[z\_] := function but patching up a hole (removable discontinuity, e.g.  $(E^x-1)/x$  at  $x=0$ ).

functionInterval[z\_] := Evaluating function with interval arithmetic.

See the examples below.

## The functions Q, Q', and QInverse

```
In[ ]:= Q[z_] := 
$$\frac{z (E^z - 1)}{E^z - 1 - z}$$

QSymb = Inactive[Q];
QContinuous[z_] := If[Abs[z] < 2^(-100), 2 +  $\frac{z}{3}$ , Q[z]]
QInterval[z_Interval] := monotoneFuncInterval[QContinuous, z]
```

```
In[ ]:= QDerivative[x_] := 
$$\frac{1 + e^{2x} - e^x (2 + x^2)}{(1 - e^x + x)^2}$$

QDerivativeSymb = Inactive[QDerivative];
QDerivativeInterval[x_Interval] := monotoneFuncInterval[QDerivative, x]
```

```
In[ ]:= Plot[Q[z], {z, -10, 10}]
```

Out[ ]:=

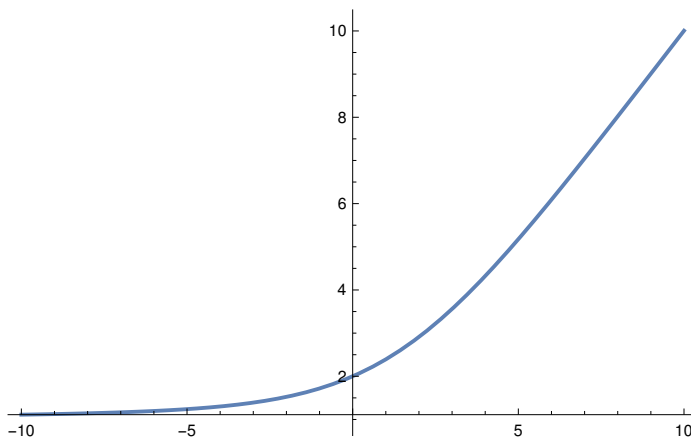

```
In[ ]:= QInverse[v_Real] := (z /. First@FindRoot[Q[z] == v, {z, 1}])
QInverse[v_Integer] := QInverse[N@v]
```

```
In[ ]:= QInverse[3.0]
```

```
Out[ ]:= 2.14913
```

```
In[ ]:= QInverse[2.1]
```

```
Out[ ]:= 0.286104
```

```
In[ ]:= QInverse[2.00001]
```

```
Out[ ]:= 0.0000306846
```

## Various rational functions involving $E^z$ , such as expProd

```
In[ ]:= expProd[z_] := (E^z - 1) z
expProdSymb = Inactive[expProd];
(* expProd is decreasing until 0 and then increasing *)
expProdInterval[z_Interval] := bimonotoneFuncInterval[expProd, z, 0]
expProdInterval[z_Real] := expProdInterval[Interval@z]
expProdDerivative[z_] := E^z (z + 1) - 1
expProdDerivativeInterval[z_Interval] := monotoneFuncInterval[expProdDerivative, z]
expProdDerivativeInterval[z_Real] := expProdDerivativeInterval[Interval@z]
expProdDerivativeDerivative[z_] := E^z (2 + z)
expProdDerivativeDerivativeInterval[z_Interval] :=
  monotoneFuncInterval[expProdDerivativeDerivative, z]
expProdDerivativeDerivativeInterval[z_Real] :=
  expProdDerivativeDerivativeInterval[Interval@z]
```

```
In[ ]:= Plot[expProd[z], {z, -2, 2}]
```

```
Out[ ]:=
```

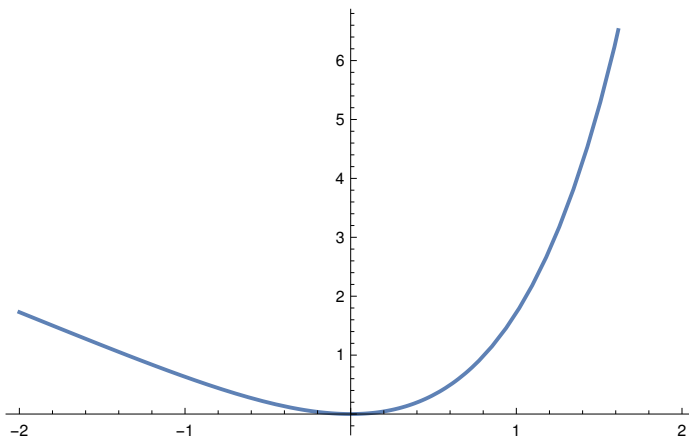

```

In[ ]:= expProdOverZSquared[z_] := 
$$\frac{E^z - 1}{z}$$

expProdOverZSquaredContinuous[z_] := If[z == 0, 1, expProdOverZSquared[z]]
expProdOverZSquaredInterval[z_Interval] :=
  monotoneFuncInterval[expProdOverZSquaredContinuous, z]
expProdOverZSquaredInterval[z_Real] := expProdOverZSquaredInterval[z]
expProdOverZSquaredSymb = Inactive[expProdOverZSquared];

expProdDerivativeOverZ[z_] := 
$$\frac{E^z (z + 1) - 1}{z}$$

expProdDerivativeOverZContinuous[z_] := If[z == 0, 2, expProdDerivativeOverZ[z]]
expProdDerivativeOverZInterval[z_Interval] :=
  monotoneFuncInterval[expProdDerivativeOverZContinuous, z]
expProdDerivativeOverZInterval[z_Real] := expProdDerivativeOverZInterval[z]
expProdDerivativeOverZSymb = Inactive[expProdDerivativeOverZ];

```

```

In[ ]:= Plot[expProdOverZSquared[z], {z, -5, 5}]

```

Out[ ]:=

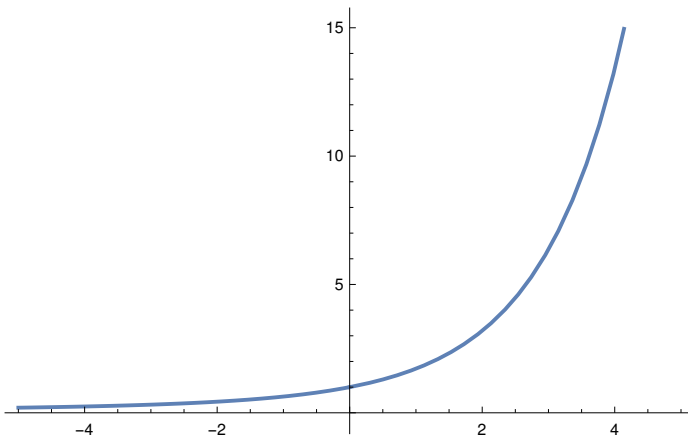

```

In[ ]:= expM2[z_] := E^z - 1 - z
expM2Interval[z_Interval] := bimonotoneFuncInterval[expM2, z, 0]
expM2Symb = Inactive[expM2];

```

In[ ]:= Plot[expM2[z], {z, -3, 3}]

Out[ ]:=

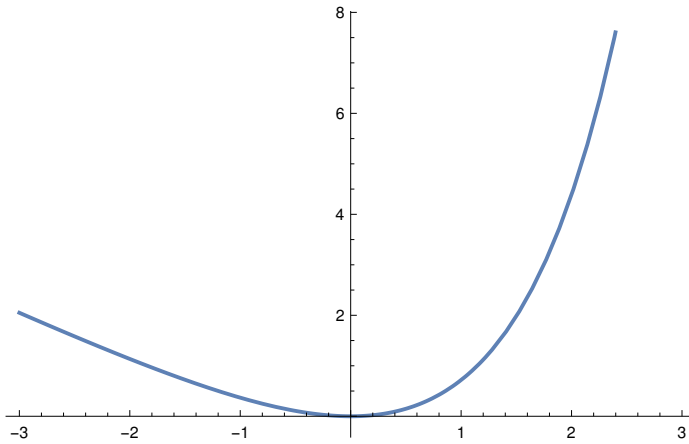

In[ ]:=

$$\text{expM2overZSquared}[z\_]:= \frac{E^z - 1 - z}{z^2}$$

$$\text{expM2overZSquaredContinuous}[z\_]:= \text{If}[\text{Abs}[z] < 2^{(-100)}, \frac{1}{2} + \frac{z}{6}, \text{expM2overZSquared}[z]]$$

$$\text{expM2overZSquaredInterval}[z\_Interval] :=$$

$$\text{monotoneFuncInterval}[\text{expM2overZSquaredContinuous}, z]$$

$$\text{expM2overZSquaredSymb} = \text{Inactive}[\text{expM2overZSquared}];$$

In[ ]:= Plot[expM2overZSquared[z], {z, -5, 5}]

Out[ ]:=

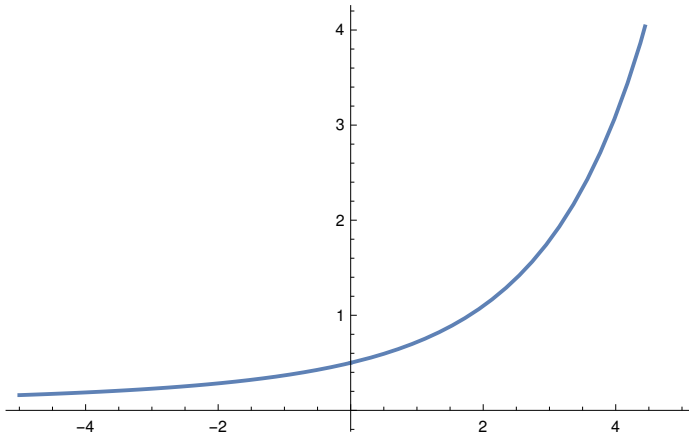

In[ ]:=

$$\text{expXm}[x\_]:= E^x (x - 1)$$

$$\text{expXmInterval}[x\_Interval] := \text{bimonotoneFuncInterval}[\text{expXm}, x, 0]$$

$$\text{expXmSymb} = \text{Inactive}[\text{expXm}];$$

In[ ]:=

$$\text{expXmx}[x\_]:= E^x x$$

$$\text{expXmxInterval}[x\_Interval] := \text{bimonotoneFuncInterval}[\text{expXmx}, x, -1]$$

$$\text{expXmxSymb} = \text{Inactive}[\text{expXmx}];$$

## nxLog and entropy H

In[ ]:= **Ln = Log;**

In[ ]:= **nxLog[z\_] := -z Log[z]  
 nxLogSymb = Inactive[nxLog];  
 nxLogContinuous[z\_] := If[z == 0, 0, nxLog[z]]  
 nxLogInterval[z\_Interval] := bimonotoneFuncInterval[nxLogContinuous, z, 1/E]**

In[ ]:= **Plot[nxLog[x], {x, 0, 1}]**

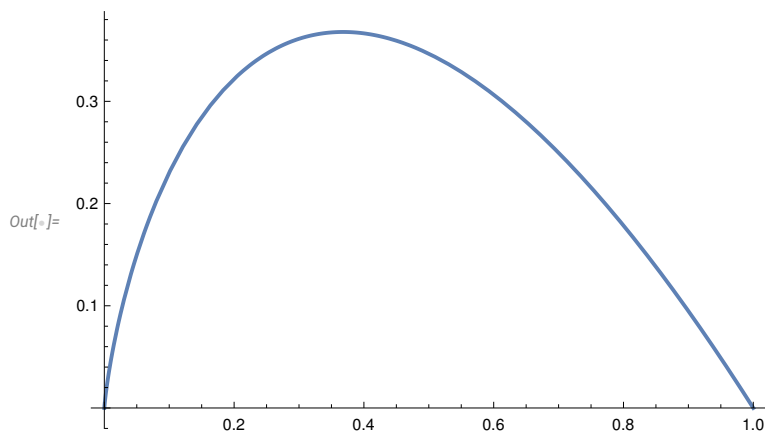

In[ ]:= **H[z\_] := nxLog[z] + nxLog[1 - z]  
 HSymb = Inactive[H];  
 HInterval[z\_Interval] := bimonotoneFuncInterval[H, z, 1/2]**

In[ ]:= **Plot[H[x], {x, 0, 1}]**

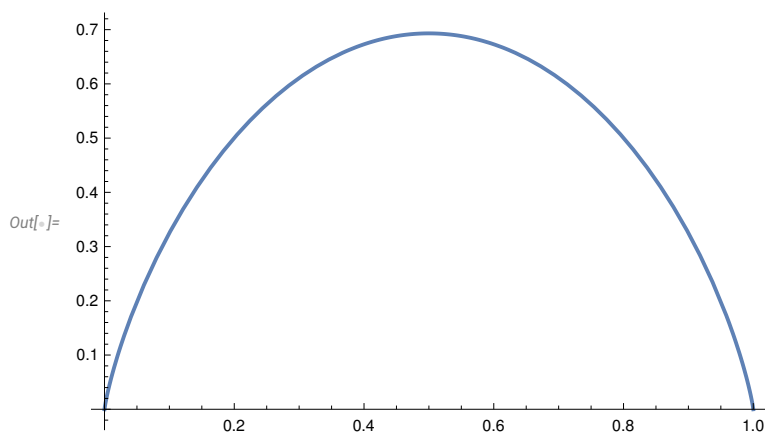

Helper to convert special symbolic functions to interval

## arithmetic functions.

We manipulate expressions in symbolic form, but for final evaluation, they need to be converted to handle interval arithmetic well. An example is provided after the definition -- using the `symbToInterval` form makes the result interval much narrower than naive evaluation, while still being correct.

```
In[ ]:= symbToIntervalNoMultiply[e_] := e /. {
  QSymb → QInterval, QSymb' → QDerivativeInterval,
  expProdSymb → expProdInterval, expProdSymb' → expProdDerivativeInterval,
  expProdSymb' → expProdDerivativeDerivativeInterval,
  multiplySymb → multiplyInterval,
  expProdOverZSquaredSymb → expProdOverZSquaredInterval,
  expProdDerivativeOverZSymb → expProdDerivativeOverZInterval,
  expM2Symb → expM2Interval,
  expM2OverZSquaredSymb → expM2OverZSquaredInterval,
  HSymb → HInterval,
  nxLogSymb → nxLogInterval,
  expXmSymb → expXmInterval,
  expXmxSymb → expXmxInterval
}
symbToInterval[e_] := symbToIntervalNoMultiply[e] //. {x_ y_ → multiplyInterval[x, y]}
```

```
In[ ]:= (* Example usage *)
exprDemo = QSymb[x] + QSymb'[x] + expProdSymb[x]
Activate[exprDemo] /. x → Interval[{0.1, 0.1001}]
symbToInterval[exprDemo]
symbToInterval[exprDemo] /. x → Interval[{0.1, 0.1001}]
Activate[exprDemo] /. x → 0.10005
```

```
Out[ ]:= expProd[x] + Q[x] + Q'[x]
```

```
Out[ ]:= Interval[{-0.307677, 5.01492}]
```

```
Out[ ]:= expProdInterval[x] + QDerivativeInterval[x] + QInterval[x]
```

```
Out[ ]:= Interval[{2.38896, 2.38903}]
```

```
Out[ ]:= 2.389
```

## Evaluating $c^*_K$ at a few points (Table 1.1, \Cref{tab:nb-computed-cThreshK})

```
In[ ]:= hK[μ_, K_] := 
$$\frac{\mu}{(E^\mu - \mu (E^\mu - 1))^{K-1}}$$

cThreshK[K_] := hK[QInverse[K], K]
```

```
In[ ]:= Table[cThreshK[K], {K, 3, 10}]
```

```
Out[ ]:= {2.75381, 3.90708, 4.96219, 5.98428, 6.99345, 7.99728, 8.99888, 9.99954}
```

```
In[ ]:= Table[cThreshK[K] / K, {K, 3, 10}]
```

```
Out[ ]:= {0.917935, 0.97677, 0.992438, 0.99738, 0.999064, 0.99966, 0.999876, 0.999954}
```

```
In[ ]:= DiscretePlot[cThreshK[K] / K, {K, 3, 10}]
```

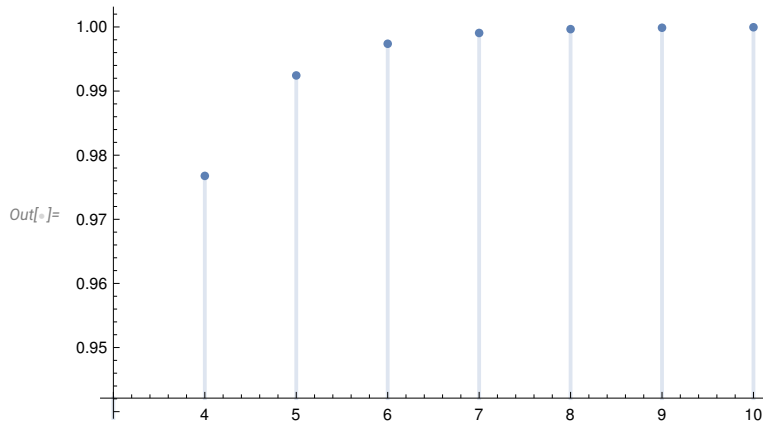

## Interval arithmetic towards proving $J_K < -\varepsilon$ for $2 < c < K$ .

Interval arithmetic calculations are used here for  $K=3$  (along  $\zeta=\zeta_{\text{sqrt}}$ ) and  $K=4,5,6$  (along  $\zeta=\zeta_{\text{lin}}$ ) to show  $J_K < -\varepsilon$  along different regions of  $(\alpha, c)$ .

The paper “The Satisfiability Threshold for  $K$ -XOR Games” integrates these calculations into a cohesive argument to show  $J_K < -\varepsilon$  along much larger regions of  $(\alpha, c)$  for all  $K \geq 3$ .

# Definitions of J\_K, L\_K, ζlin, ζsqrt, and related functions

## Definitions

In[ ]:= JK[α\_, ζ1\_, ζ2\_, c\_, K\_] := With[{λ = QInverse[c]},  

$$\frac{1}{K} H[\alpha] + \alpha \operatorname{Log}[\alpha / \zeta 1] + (1 - \alpha) \operatorname{Log}[(1 - \alpha) / \zeta 2] + \frac{1}{c} \operatorname{Log}\left[\frac{\exp M2[\lambda (\zeta 2 + \zeta 1)] + \exp M2[\lambda (\zeta 2 - \zeta 1)]}{2 \exp M2[\lambda]}\right]$$
  
 ]  
 JK[α\_, ζ\_List, c\_, K\_] := JK[α, ζ[[1]], ζ[[2]], c, K]

In[ ]:= JKλ[α\_, ζ1\_, ζ2\_, λ\_, K\_] :=  

$$\frac{1}{K} H[\alpha] + \alpha \operatorname{Log}[\alpha / \zeta 1] + (1 - \alpha) \operatorname{Log}[(1 - \alpha) / \zeta 2] + \frac{1}{Q[\lambda]} \operatorname{Log}\left[\frac{\exp M2[\lambda (\zeta 2 + \zeta 1)] + \exp M2[\lambda (\zeta 2 - \zeta 1)]}{2 \exp M2[\lambda]}\right]$$
  
 JKλ[α\_, ζ\_List, λ\_, K\_] := JKλ[α, ζ[[1]], ζ[[2]], λ, K]

In[ ]:= JKλSymb = 
$$\frac{1}{K} H[\alpha] + \alpha \operatorname{Log}[\alpha / \zeta 1] + (1 - \alpha) \operatorname{Log}[(1 - \alpha) / \zeta 2] +$$
  

$$\frac{1}{Q\text{Symb}[\lambda]} \operatorname{Log}\left[\frac{\exp M2\text{Symb}[\lambda (\zeta 2 + \zeta 1)] + \exp M2\text{Symb}[\lambda (\zeta 2 - \zeta 1)]}{2 \exp M2\text{Symb}[\lambda]}\right]$$

Out[ ]:= 
$$\frac{(-1 + \alpha) \operatorname{Log}[1 - \alpha] - \alpha \operatorname{Log}[\alpha]}{K} + \alpha \operatorname{Log}\left[\frac{\alpha}{\zeta 1}\right] + (1 - \alpha) \operatorname{Log}\left[\frac{1 - \alpha}{\zeta 2}\right] + \frac{\operatorname{Log}\left[\frac{\exp M2[(-\zeta 1 + \zeta 2) \lambda] + \exp M2[(\zeta 1 + \zeta 2) \lambda]}{2 \exp M2[\lambda]}\right]}{Q[\lambda]}$$

In[ ]:= ζsqrtα\_, K\_] := {Sqrt[α / (K - 1)], 1 - α};  
 ζsqrtReflectα\_, K\_] := If[α < 1 / 2, ζsqrtα, K], With[{ζ = ζsqrt[1 - α, K]}, {ζ[[2]], ζ[[1]]}]  
 ζlin[α\_] := {α, 1 - α};



```
In[ ]:= Plot[{ζLin[α][1], ζLin[α][2]}, {α, 0, 1}]
```

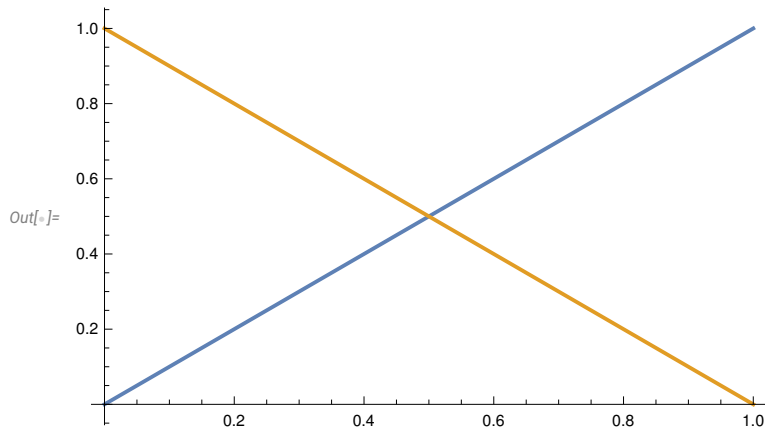

```
In[ ]:= Plot[{ζSqrt[α, 3][1], ζSqrt[α, 3][2]}, {α, 0, 1}]
```

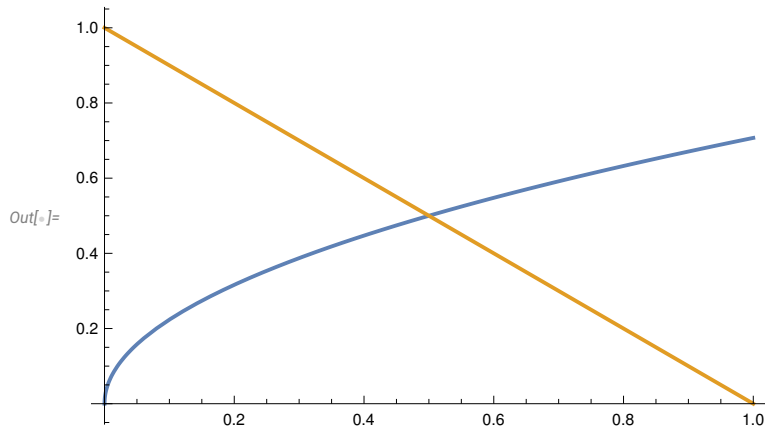

Symbolic definition of  $J_K$  at  $\zeta_{\text{Lin}}(J_{K\text{Lin}} = L_K/c)$

```
In[ ]:= JKLIn[α_, λ_, K_] := JKλ[α, ζLin[α], λ, K]
```

```
In[ ]:= JKLInSymb = JKλSymb /. {ζ1 → α, ζ2 → 1 - α}
```

$$\text{Out[ ]} = \frac{(-1 + \alpha) \text{Log}[1 - \alpha] - \alpha \text{Log}[\alpha]}{K} + \frac{\text{Log}\left[\frac{\exp M2[\lambda] + \exp M2[(1-2\alpha)\lambda]}{2 \exp M2[\lambda]}\right]}{Q[\lambda]}$$

```
In[ ]:= JKLIn[α_, c_, K_] := JKLIn[α, QInverse[c], K]
```

```
In[ ]:= Plot[JKLin[α, 3.99999, 4], {α, 0.45, 0.55}]
```

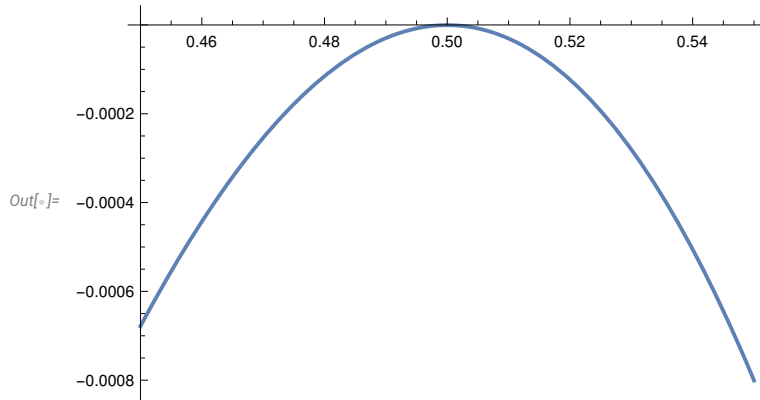

## Symbolic definition of J\_K at ζsqrt

```
In[ ]:= (* ζ = ζsqrt = {Sqrt[α/(K-1)], 1-α} *)
JKSqrt[α_, c_, K_] := JK[α, ζsqrt[α, K], c, K]
J3Sqrt[α_, c_] := JKSqrt[α, c, 3]
JKSqrtλ[α_, λ_, K_] := JKλ[α, ζsqrt[α, K], λ, K]
J3Sqrtλ[α_, λ_] := JKSqrtλ[α, λ, 3]
```

```
In[ ]:= J3SqrtλSymb = JKλSymb /. {ζ1 → Sqrt[α/2], ζ2 → 1-α, K → 3};
cJ3SqrtλSymb = FullSimplify[QSymb[λ] * J3SqrtλSymb];
```

```
In[ ]:= cJ3SqrtλSymb2 = FullSimplify[cJ3SqrtλSymb /. {expM2 → expM2}]
```

$$\text{Out[ ]} = \text{Log}\left[\frac{1 + \lambda - \alpha \lambda - e^{\lambda - \alpha \lambda} \text{Cosh}\left[\frac{\sqrt{\alpha} \lambda}{\sqrt{2}}\right]}{1 - e^{\lambda} + \lambda}\right] + \frac{1}{6} \left(2(-1 + \alpha) \text{Log}[1 - \alpha] + \alpha \text{Log}[8 \alpha]\right) Q[\lambda]$$

```
In[ ]:= cJ3SqrtλSymb3 = Log[
$$\frac{1 + \lambda(1 - \alpha) - e^{\lambda(1 - \alpha)} \text{Cosh}\left[\frac{\sqrt{\alpha} \lambda}{\sqrt{2}}\right]}{1 - e^{\lambda} + \lambda}$$
] + 
$$\frac{1}{6} (-2(1 - \alpha) \text{Log}[1 - \alpha] + \alpha \text{Log}[8 \alpha]) Q[\lambda];$$

(* Testing that cJ3SqrtλSymb2 == cJ3SqrtλSymb3 *)
Simplify[cJ3SqrtλSymb3 - cJ3SqrtλSymb2]
```

```
Out[ ]:= 0
```

## Taking derivative with respect to $\alpha$

In[ ]:= `d$CJ3sqrt$α = Simplify[Dt[cJ3SqrtλSymb, α] /. {Dt[λ, α] → 0, expM2'[x_] → E^x - 1}]`

$$\text{Out[ ]} = \frac{\left(8 + e^{\lambda - \frac{\sqrt{\alpha}\lambda}{\sqrt{2}} - \alpha\lambda} \left(-4 - \frac{\sqrt{2}}{\sqrt{\alpha}}\right) + e^{\lambda + \frac{\sqrt{\alpha}\lambda}{\sqrt{2}} - \alpha\lambda} \left(-4 + \frac{\sqrt{2}}{\sqrt{\alpha}}\right)\right)\lambda}{4 \left(\expM2\left[\lambda - \frac{\sqrt{\alpha}\lambda}{\sqrt{2}} - \alpha\lambda\right] + \expM2\left[\lambda + \frac{\sqrt{\alpha}\lambda}{\sqrt{2}} - \alpha\lambda\right]\right)} + \frac{1}{6} (3 + 2 \text{Log}[1 - \alpha] + \text{Log}[8 \alpha]) Q[\lambda]$$

In[ ]:= `d$CJ3sqrt$αα = Simplify[Dt[d$CJ3sqrt$α, α] /. {Dt[λ, α] → 0, expM2'[x_] → E^x - 1}]`

$$\text{Out[ ]} = - \frac{e^{-\sqrt{2}\sqrt{\alpha}\lambda - 2\alpha\lambda} \left( e^{\lambda + \sqrt{2}\sqrt{\alpha}\lambda} (\sqrt{2} - 4\sqrt{\alpha}) - e^{\lambda} (\sqrt{2} + 4\sqrt{\alpha}) + 8 e^{\frac{\sqrt{\alpha}\lambda}{\sqrt{2}} + \alpha\lambda} \sqrt{\alpha} \right)^2 \lambda^2}{16 \alpha \left( \expM2\left[\lambda - \frac{\sqrt{\alpha}\lambda}{\sqrt{2}} - \alpha\lambda\right] + \expM2\left[\lambda + \frac{\sqrt{\alpha}\lambda}{\sqrt{2}} - \alpha\lambda\right] \right)^2} +$$

$$\frac{e^{\lambda - \frac{\sqrt{\alpha}\lambda}{\sqrt{2}} - \alpha\lambda} \lambda \left( \sqrt{2} + \sqrt{\alpha}\lambda + 4\sqrt{2}\alpha\lambda + 8\alpha^{3/2}\lambda + e^{\sqrt{2}\sqrt{\alpha}\lambda} (-\sqrt{2} + \sqrt{\alpha}\lambda - 4\sqrt{2}\alpha\lambda + 8\alpha^{3/2}\lambda) \right)}{8\alpha^{3/2} \left( \expM2\left[\lambda - \frac{\sqrt{\alpha}\lambda}{\sqrt{2}} - \alpha\lambda\right] + \expM2\left[\lambda + \frac{\sqrt{\alpha}\lambda}{\sqrt{2}} - \alpha\lambda\right] \right)} + \frac{(-1 + 3\alpha) Q[\lambda]}{6(-1 + \alpha)\alpha}$$

## Exact simplification of J\_3 at $\zeta\text{sqrt}$ and $\alpha = 1/2$

Exact simplification at  $\alpha = 1/2$

Conclusion:  $0 = \partial_{\alpha} c J3\text{sqrt}$  at  $\alpha = 1/2$  for all  $\lambda$ .  
(Equation 4.3.1, \Cref{eq:nb-4-Jsqrt3-at-half})

In[ ]:= `Simplify[Activate[d$CJ3sqrt$α /. {α → 1/2}]]`

Out[ ]:= 0

More exact simplification at  $\alpha = 1/2$ .

Conclusion:  $c J3\text{sqrt} = (1/3) (c-3) \ln(2)$  when  $\alpha = 1/2$ .  
(Equation 4.3.1, \Cref{eq:nb-4-Jsqrt3-at-half})

In[ ]:= `Simplify[cJ3SqrtλSymb2 /. {α → 1/2, Q[λ] → c}]`

$$\text{Out[ ]} = \frac{1}{3} (-3 + c) \text{Log}[2]$$

## Interval definition of J\_3 ( $\zeta\text{sqrt}$ )

In[ ]:= **cJ3Sqrt** $\lambda$ Symb

$$\text{Out[ ]}:= \text{Log}\left[\frac{\exp M2\left[\lambda - \frac{\sqrt{\alpha}}{\sqrt{2}} - \alpha\lambda\right] + \exp M2\left[\lambda + \frac{\sqrt{\alpha}}{\sqrt{2}} - \alpha\lambda\right]}{2 \exp M2[\lambda]}\right] + \frac{1}{6} \left(2(-1 + \alpha) \text{Log}[1 - \alpha] + \alpha \text{Log}[8 \alpha]\right) \mathbb{Q}[\lambda]$$

In[ ]:= **Simplify**[ $\exp M2[x] - x^2 \exp M2\text{overZSquared}[x]$ ]

Out[ ]:= 0

In[ ]:= **cJ3Sqrt** $\lambda$ SymbForInterval = **FullSimplify**[  
**cJ3Sqrt** $\lambda$ Symb /. {**expM2**[x\_]  $\rightarrow$  x<sup>2</sup> \* **expM2overZSquaredSymb**[x]}  
 1

$$\text{Out[ ]}:= \text{Log}\left[\frac{\left(-1 + \frac{\sqrt{\alpha}}{\sqrt{2}} + \alpha\right)^2 \exp M2\text{overZSquared}\left[\lambda - \frac{\sqrt{\alpha}}{\sqrt{2}} - \alpha\lambda\right] + \left(1 + \frac{\sqrt{\alpha}}{\sqrt{2}} - \alpha\right)^2 \exp M2\text{overZSquared}\left[\lambda + \frac{\sqrt{\alpha}}{\sqrt{2}} - \alpha\lambda\right]}{2 \exp M2\text{overZSquared}[\lambda]}\right] +$$

$$\frac{1}{6} \left(2(-1 + \alpha) \text{Log}[1 - \alpha] + \alpha \text{Log}[8 \alpha]\right) \mathbb{Q}[\lambda]$$

In[ ]:= **cJ3Sqrt** $\lambda$ IntervalSymb = **symbToInterval**@**cJ3Sqrt** $\lambda$ SymbForInterval;  
**cJ3Sqrt** $\lambda$ Interval[ $\alpha_0$ \_,  $\lambda_0$ \_] := **AllowUnderflow**[**cJ3Sqrt** $\lambda$ IntervalSymb /. { $\alpha \rightarrow \alpha_0$ ,  $\lambda \rightarrow \lambda_0$ }]

In[ ]:= **d** $\zeta$ **J3sqrt** $\alpha\alpha$ IntervalSymb = **symbToIntervalNoMultiply**@**d** $\zeta$ **J3sqrt** $\alpha\alpha$ ;  
**d** $\zeta$ **J3sqrt** $\alpha\alpha$ Interval[ $\alpha_0$ \_,  $\lambda_0$ \_] :=  
**AllowUnderflow**[**d** $\zeta$ **J3sqrt** $\alpha\alpha$ IntervalSymb /. { $\alpha \rightarrow \alpha_0$ ,  $\lambda \rightarrow \lambda_0$ }]

## Plots of $J_3(\zeta\sqrt{\alpha})$

```
In[ ]:= (*
J3 at  $\zeta\sqrt{\alpha}$ . This suggests  $J_3 \zeta\sqrt{\alpha} \leq 0$ ,
with equality holding at  $\alpha=0$  and at  $(\alpha=1/2 \text{ and } c=3 \text{ (so } \lambda \approx 2.149))$ .
*)
Plot3D[J3Sqrt $\lambda[\alpha, \lambda]$ , { $\alpha$ , 0, 1/2}, { $\lambda$ , 0.0001, 2.149}, AxesLabel → Automatic]
```

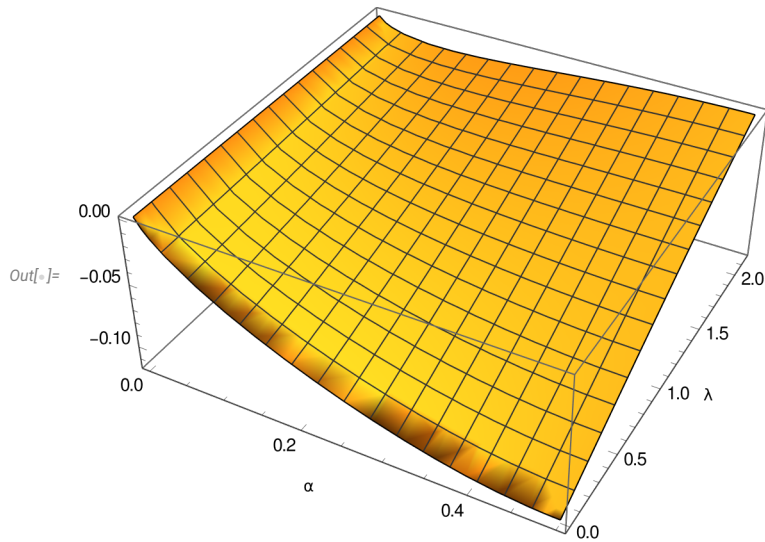

```
In[ ]:= (*
Note J3( $\alpha, \zeta\sqrt{\alpha}, c$ )>
0 for  $\alpha$  close to 1 and  $c$  close to 2. That's why we reflect after  $\alpha=0.5$ .
*)
Plot[{J3Sqrt[ $\alpha$ , 3], J3Sqrt[ $\alpha$ , 2.7], J3Sqrt[ $\alpha$ , 2.4], J3Sqrt[ $\alpha$ , 2.1]}, { $\alpha$ , 0, 1},
AxesLabel → Automatic, PlotLegends → {"c=3", "c=2.7", "c=2.4", "c=2.1"}]
```

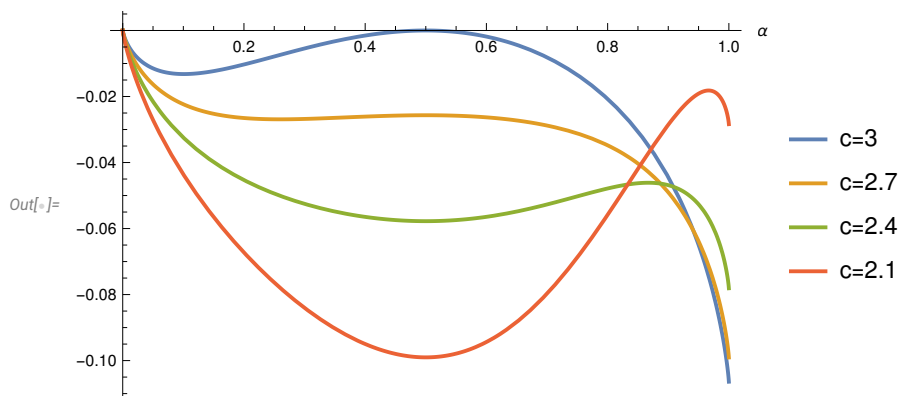

## Interval definitions J\_K( $\zeta$ lin)

In[ ]:= JKLInSymb

$$\text{Out[ ]} = \frac{(-1 + \alpha) \text{Log}[1 - \alpha] - \alpha \text{Log}[\alpha]}{K} + \frac{\text{Log}\left[\frac{\exp M2[\lambda] + \exp M2[(1 - 2\alpha)\lambda]}{2 \exp M2[\lambda]}\right]}{Q[\lambda]}$$

In[ ]:= JKLInSymbForInterval =  $\frac{\text{HSymb}[\alpha]}{K} + \frac{\text{Log}\left[\frac{\exp M2[\lambda] + \exp M2[(1 - 2\alpha)\lambda]}{2 \exp M2[\lambda]}\right]}{Q[\lambda]}$  ;  
Simplify[Activate[JKLInSymbForInterval - JKLInSymb]]

Out[ ]:= 0

In[ ]:= JKLInIntervalSymb = symbToInterval@JKLInSymbForInterval;  
JKLInInterval[ $\alpha_0$ ,  $\lambda_0$ ,  $K_0$ ] :=  
AllowUnderflow[JKLInIntervalSymb /. { $\alpha \rightarrow \alpha_0$ ,  $\lambda \rightarrow \lambda_0$ ,  $K \rightarrow K_0$ }]

## Plots of J\_K( $\zeta$ lin)

In[ ]:= JKLInCK[ $\alpha$ , K\_] := JKLIn[ $\alpha$ , K, K]

JKLin for  $c=K$ , for  $K=4,5,6$ .  
(Figure 4.1, \Cref{fig:nb-Jklin456})

In[ ]:= JKlinSlice[ $\alpha$ , K\_] := If[ $\alpha > 0.99 \beta K[K]$ , JKLInCK[ $\alpha$ , K]  
Plot[{JKlinSlice[ $\alpha$ , 4], JKlinSlice[ $\alpha$ , 5], JKlinSlice[ $\alpha$ , 6]},  
{ $\alpha$ , 0.1, 1}, AxesLabel -> {" $\alpha$ "}, PlotLabels -> {"K=4", "K=5", "K=6"}]

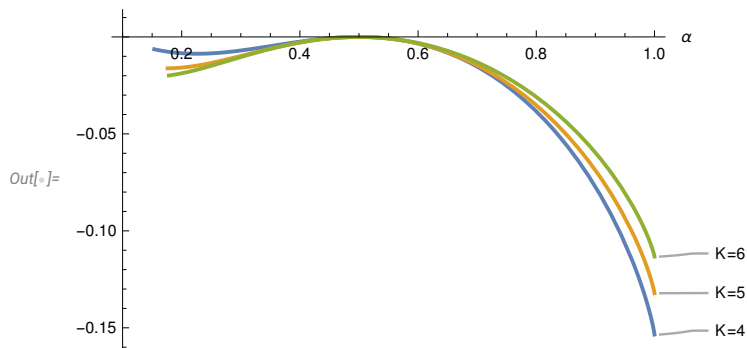

JKLin for  $K=4$ , for varying  $c$ .

(Figure 4.2, \Cref{nb-JKLin\_K4\_varying\_c})

```
In[ ]:= JKLinK4Slice[α_, c_] := With[{K = 4}, If[α > 0.99 β[K], JKLin[α, c, K]]]
Plot[{JKLinK4Slice[α, 2.02], JKLinK4Slice[α, 2.1],
      JKLinK4Slice[α, 2.3], JKLinK4Slice[α, 2.6], JKLinK4Slice[α, 2.99]}, {α, 0.1, 1},
  AxesLabel → {"α"}, PlotLabels → {"c=2.02", "c=2.1", "c=2.3", "c=2.6", "c=2.99"}]
```

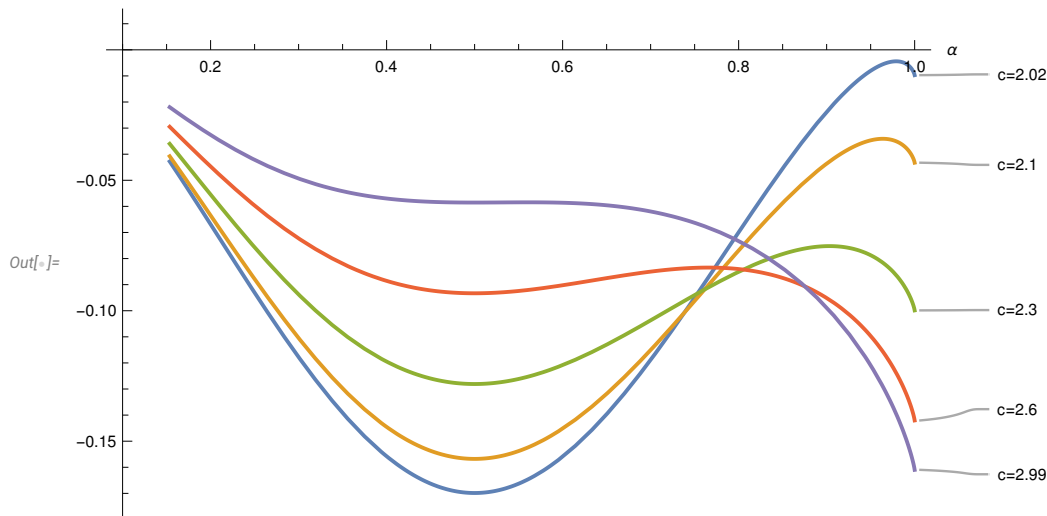

Misc plots for  $c=K$

```
In[ ]:= (* This is why we can't handle K=3 with primarily JKLin *)
With[{K = 3}, Plot[JKLinCK[α, K], {α, 0.99 β[K], 1}, AxesLabel → {"α"}]]
```

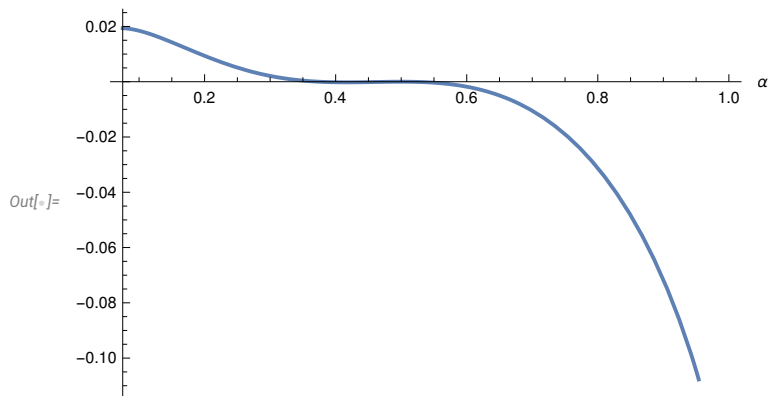

```
In[ ]:= With[{K = 4}, Plot[JKLinCK[α, K], {α, 0.99 βK[K], 1}, AxesLabel → {"α"}]]
```

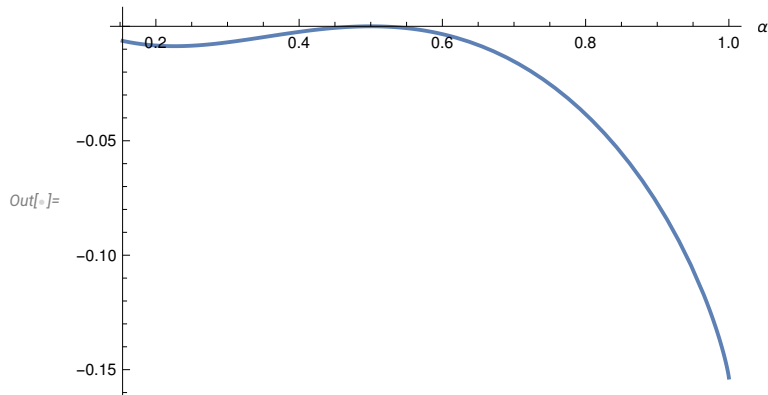

```
In[ ]:= With[{K = 5}, Plot[JKLinCK[α, K], {α, 0.99 βK[K], 1}, AxesLabel → {"α"}]]
```

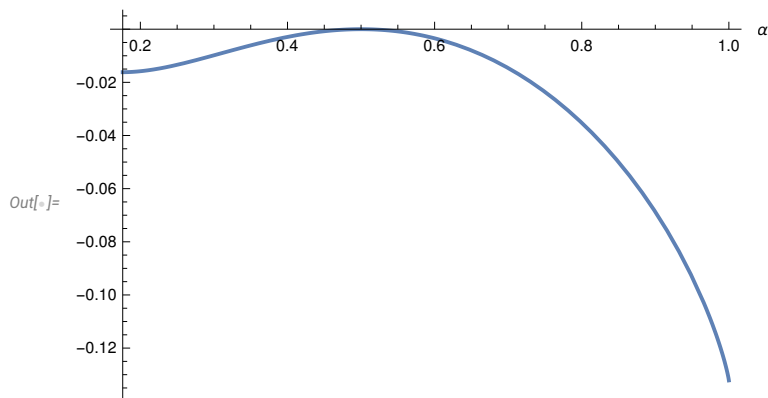

## Defining and analyzing $\beta_K$ , $\alpha_K$ , and $\alpha_K^*$

Definition of  $\beta_K$ ,  $\alpha_K$ ,  $\alpha_K^*$

```
In[ ]:= βK[k_] := Exp[- $\frac{\frac{1}{k} + \text{Log}[\text{Sqrt}[k - 1]] - 1 + \frac{k}{2(k-1)}}{\frac{1}{2} - \frac{1}{k}}$ ]
```

```
In[ ]:= αK[k_] := E k ^ (-k / (k - 2))
```

```
In[ ]:= αKStar[k_] := With[{λk = QInverse[k]},  $\frac{1}{2} \left( 1 - \frac{1}{\lambda k} \text{Log}\left[\frac{\text{expM2}[\lambda k]}{\lambda k^2}\right] \right)$ ]
```

```
In[ ]:= βK[3.0]
```

```
Out[ ]:= 0.0758163
```



In[ ]:= DiscretePlot[{ $\beta_k[k]$ }, {k, 3, 50}, PlotLabels  $\rightarrow$  " $\beta_K$ "]

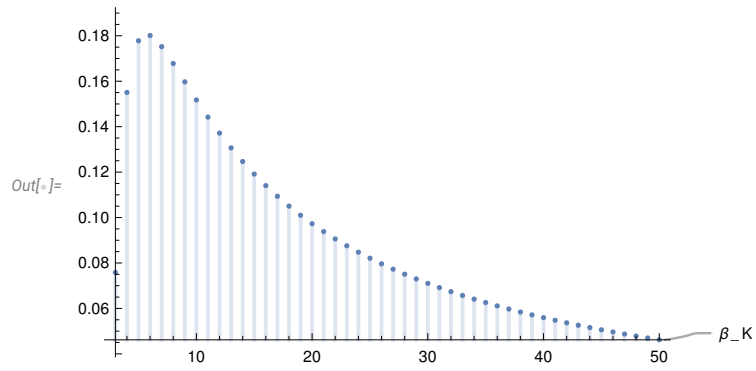

In[ ]:= DiscretePlot[{ $K \beta_k[k]$ }, {K, 3, 50}, PlotLabels  $\rightarrow$  " $K \beta_K$ "]

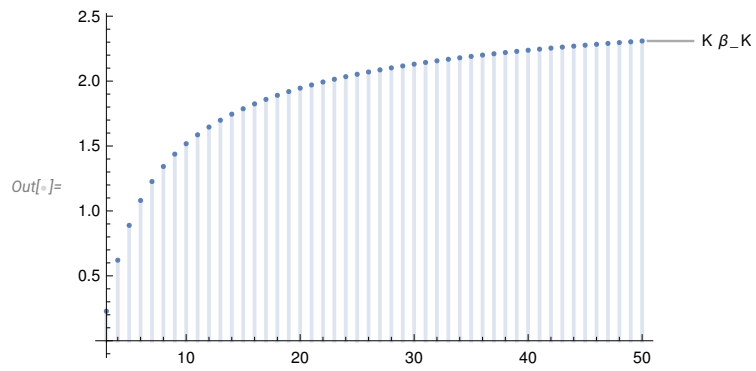

In[ ]:= DiscretePlot[{ $\text{Log}[\beta_k[k] / (E^{k(-k/(k-2))})]$ }, {k, 3, 20}, PlotLegends  $\rightarrow$  {" $\beta_k$ ", " $\alpha_k$ "}]

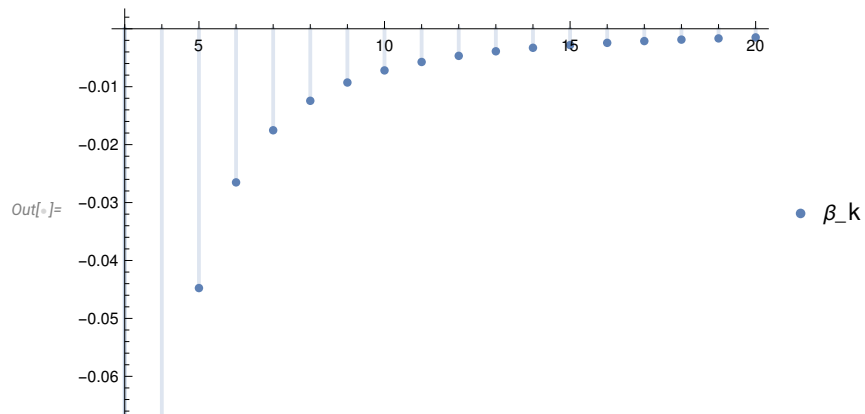

## Differentiation of $K^*\beta_K$

Conclusion:  $K^*\beta_K$  is increasing for  $K \geq 4$

(Lemma 4.2.4, \Cref{lem:nb-Lk-neg-K-geq-7})

```
In[ ]:= logKβK= Simplify@PowerExpand[Log[K βK]]
```

$$\text{Out[ ]}= \frac{2 - 4K + K^2 - (-1 + K)K \log[-1 + K]}{(-2 + K)(-1 + K)} + \log[K]$$

```
In[ ]:= derivLogKβK= FullSimplify[D[logKβK, K]]
```

$$\text{Out[ ]}= \frac{4 - (-2 + K)K(-7 + 2K) + 2(-1 + K)^2K \log[-1 + K]}{K(2 - 3K + K^2)^2}$$

```
In[ ]:= (* Denominator is strictly positive for K ≥ 3. *)
Factor@Denominator[derivLogKβK]
```

$$\text{Out[ ]}= (-2 + K)^2(-1 + K)^2K$$

```
In[ ]:= Numerator[derivLogKβK]
```

$$\text{Out[ ]}= 4 - (-2 + K)K(-7 + 2K) + 2(-1 + K)^2K \log[-1 + K]$$

```
In[ ]:= p[K_] := (-2 + K)K(-7 + 2K)
q[K_] := 2(-1 + K)^2K
Simplify[Numerator[derivLogKβK] - (4 - p[K] + q[K] Log[K - 1])]
```

$$\text{Out[ ]}= 0$$

```
In[ ]:= (* q[K] - p[K] is strictly positive for K ≥ 2 *)
Factor[q[K] - p[K]]
```

$$\text{Out[ ]}= K(-12 + 7K)$$

```
In[ ]:= (* Hence for K > 1 + ε, we see the numerator is strictly positive. *)
q[K] - p[K] ≥ 0
q[K] Log[K - 1] - p[K] ≥ 0
4 - p[K] + q[K] Log[K - 1] ≥ 4
```

$$\text{Out[ ]}= 2(-1 + K)^2K - (-2 + K)K(-7 + 2K) \geq 0$$

$$\text{Out[ ]}= -((-2 + K)K(-7 + 2K)) + 2(-1 + K)^2K \log[-1 + K] \geq 0$$

$$\text{Out[ ]}= 4 - (-2 + K)K(-7 + 2K) + 2(-1 + K)^2K \log[-1 + K] \geq 4$$

## Plots: comparison of $\beta_K, \alpha_K, \alpha_K^*$

```
In[ ]:= DiscretePlot[{akStar[K], ak[K],  $\beta_K$ ], {K, 3, 20}, PlotRange → {{2.5, 20}, {0, 0.5}},
  PlotLegends → {Subscript[ $\alpha$ , K]^"*", Subscript[ $\alpha$ , K], Subscript[ $\beta$ , K]}
```

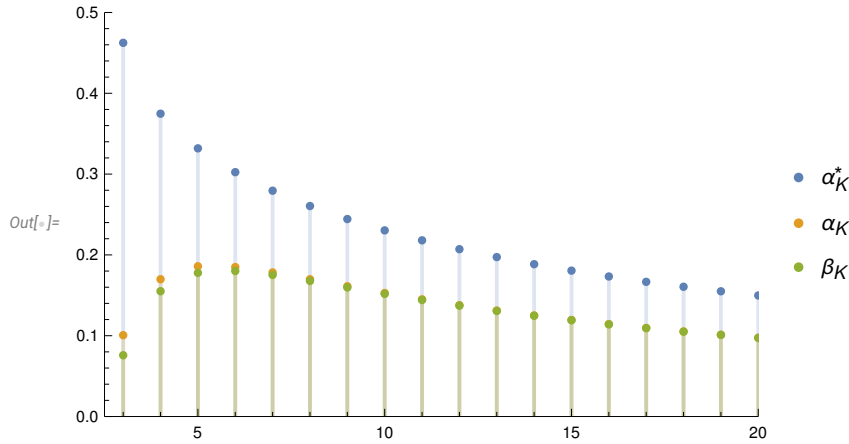

```
In[ ]:= DiscretePlot[ak[K] -  $\beta_K$ ], {K, 3, 20}]
```

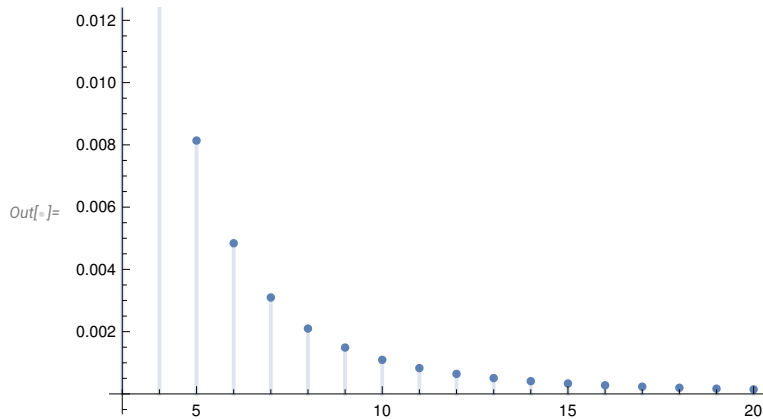

## Direct evaluation of upper bound ( $\alpha_K^*$ ) to $L_K(\alpha, K)$ (Equation 4.2.5, \Cref{eq:nb-upper-bound-LK})

```
In[ ]:= Table[akStar[k], {k, 4, 6}]
```

```
Out[ ]:= {0.374746, 0.331859, 0.302385}
```

```
In[ ]:= H[akStar[7]] + Log[ $\frac{1 + \text{Exp}[-2 * 0.99 * 7 * \beta_K[7]]}{2}$ ]
```

```
Out[ ]:= -0.0162175
```

Hence  $L_K(\alpha, K) \leq -0.0162175 < -0.016$ .

# Interval arithmetic towards $J_K(\zeta\sqrt{t}) < -\varepsilon$ for $K=3$ on regions of $(\alpha, c)$ (Lemma 4.3.1, \Cref{lem:nb-K3-Jsqrt-bound})

Gridding  $c^*J_3(\zeta\sqrt{t})$  away from  $(\alpha, c)=(0.5, 3)$

Gridding  $c^*J_3(\zeta\sqrt{t})$  (200×200 rectangles)  
Conclusion:  $cJ_3\sqrt{t} \leq -10^{-4}$  on  $[0.07, 0.5] \times [0.0, 2.0]$   
(Equation 4.3.4, \Cref{eq:nb-2a-Jsqrt3-regime})

```
In[ ]:= UniformGridPositive2DwithPicture[
  {α, λ} ↦ - ( cJ3SqrtλInterval[α, λ]
               QInterval[λ]
             + 10^-4 ),
  Interval[{0.07, 0.5}], 200,
  Interval[{0.0, 2.0}], 200
]
Problems: 0 in 1.60603s.
Success on Rectangle[{0.07, -2.22507 × 10^-308}, {0.5, 2.}]
```

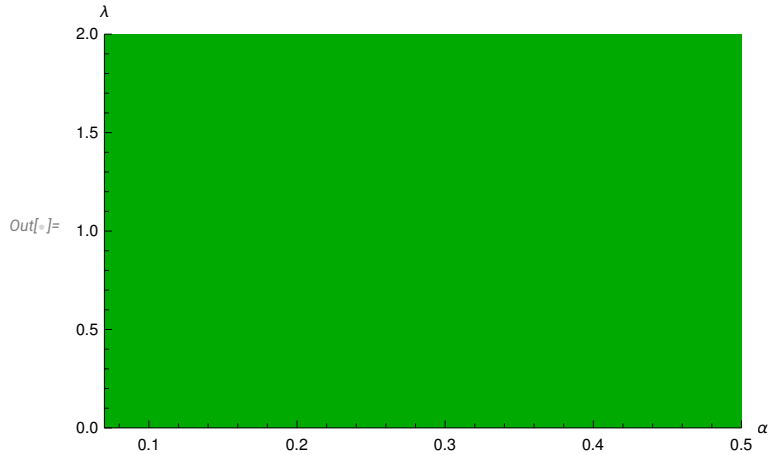

Gridding  $c^*J_3(\zeta\sqrt{t})$  (400×400 rectangles)

Conclusion:  $cJ\sqrt{t} \leq -10^{-4}$  on  $[0.07, 0.4] \times [2.0, 2.15]$

(Equation 4.3.5, \Cref{eq:nb-2b-Jsqrt3-regime})

```
In[ ]:= UniformGridPositive2DwithPicture[
  {α, λ} ↦ - (cJ3SqrtλInterval[α, λ]
    QInterval[λ]
    + 10^-4),
  Interval[{0.07, 0.40}], 400,
  Interval[{2.0, 2.15}], 400
]
Problems: 0 in 6.82912s.
Success on Rectangle[{0.07, 2.}, {0.4, 2.15}]
```

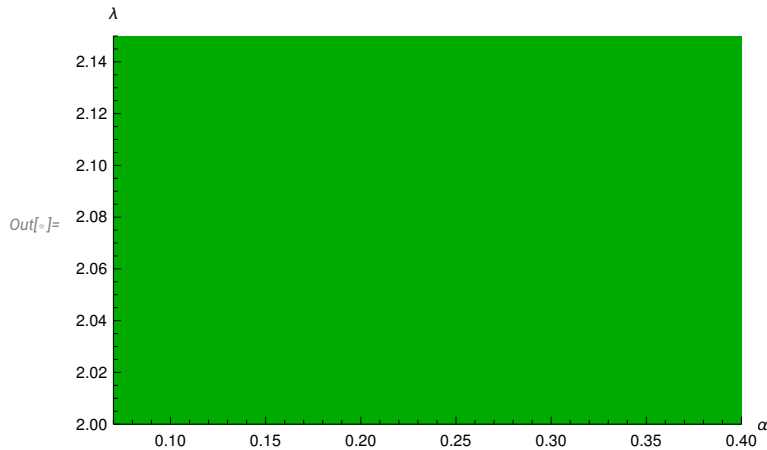

Gridding  $\partial_\alpha \partial_\alpha c^*J_3(\zeta\sqrt{t})$  near  $(\alpha, c) = (0.5, 3)$

Gridding  $\partial_\alpha \partial_\alpha cJ\sqrt{t}$  (40×40 rectangles)

Conclusion:  $\partial_\alpha \partial_\alpha cJ\sqrt{t} \leq -0.01$  on  $[0.39, 0.5] \times [1.9, 2.15]$

(Equation 4.3.2, \Cref{eq:nb-3-Jsqrt3-second-partial-alpha})

```
In[ ]:= UniformGridPositive2DwithPicture[
  {α, λ} ↦ - (d$CJ3sqrt$ααInterval[α, λ] + 0.01),
  Interval[{0.39, 0.5}], 40,
  Interval[{1.9, 2.15}], 40
]
```

Problems: 0 in 0.089878s.

Success on Rectangle[{0.39, 1.9}, {0.5, 2.15}]

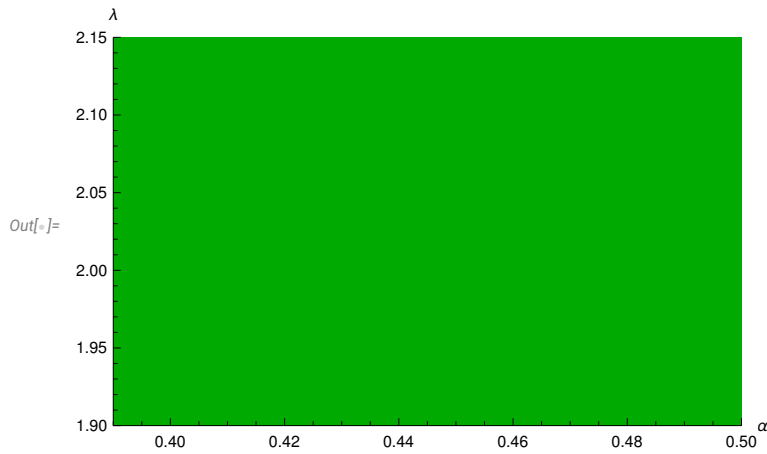

Interval arithmetic towards  $J_K(\zeta_{\text{lin}}) < -\varepsilon$  for  $K=4,5,6$  on regions of  $(\alpha, c)$   
(Lemma 4.2.3, \Cref{lem:nb-Kgeq4-J-bound})

Direct evaluation of  $\beta_K$

Conclusion:  $\beta_K > 0.15$  and  $\alpha^*_K < 0.45$  for  $K=4,5,6$ .

(Equation 4.2.3, \Cref{eq:nb-1a-beta-alpha-fits})

```
In[ ]:= {βK[4], βK[5], βK[6]} // N
```

```
Out[ ]:= {0.155068, 0.177789, 0.180116}
```

```
In[ ]:= {αkStar[4], αkStar[5], αkStar[6]} // N
```

```
Out[ ]:= {0.374746, 0.331859, 0.302385}
```

```
In[ ]:= If[0.99 βK[4] > 0.15, Print["Success: 0.99 β_4 > 0.15."]]
```

```
If[0.99 βK[5] > 0.15, Print["Success: 0.99 β_5 > 0.15."]]
```

```
If[0.99 βK[6] > 0.15, Print["Success: 0.99 β_6 > 0.15."]]
```

```
Success: 0.99 β_4 > 0.15.
```

```
Success: 0.99 β_5 > 0.15.
```

```
Success: 0.99 β_6 > 0.15.
```

```

In[ ]:=
  If[akStar[4] < 0.45, Print["Success:  $\alpha^*_4 < 0.45$ ."]]
  If[akStar[5] < 0.45, Print["Success:  $\alpha^*_5 < 0.45$ ."]]
  If[akStar[6] < 0.45, Print["Success:  $\alpha^*_6 < 0.45$ ."]]

  Success:  $\alpha^*_4 < 0.45$ .
  Success:  $\alpha^*_5 < 0.45$ .
  Success:  $\alpha^*_6 < 0.45$ .

```

## Gridding $J_K(\zeta_{lin})$

Conclusion:  $J_K(\zeta_{lin}) < -10^{-4}$  for  $c=K$  and  $0.15 \leq \alpha \leq 0.45$ , for  $K=4,5,6$ .  
(Equation 4.2.2, \Cref{eq:nb-1-LK-neg})

```

In[ ]:= With[{K = 4}, With[{c = K}, With[{ $\lambda$  = QInverse[c]},
  UniformGridPositive1DwithStatement[
     $\alpha \mapsto -(\text{JKLinInterval}[\alpha, \text{pI}@\lambda, K] + 10^{-4})$ ,
    Interval[{0.15, 0.45}], 25
  ]
]]

```

Problems: 0 in 0.031557s.

Success on Interval[{0.15, 0.45}]

```

In[ ]:=  $\beta_K[5.0]$ 

```

```

Out[ ]:= 0.177789

```

```

In[ ]:= With[{K = 5}, With[{c = K}, With[{ $\lambda$  = QInverse[c]},
  UniformGridPositive1DwithStatement[
     $\alpha \mapsto -(\text{JKLinInterval}[\alpha, \text{pI}@\lambda, K] + 10^{-4})$ ,
    Interval[{0.15, 0.45}], 25
  ]
]]

```

Problems: 0 in 0.024899s.

Success on Interval[{0.15, 0.45}]

```

In[ ]:= With[{K = 6}, With[{c = K}, With[{ $\lambda$  = QInverse[c]},
  UniformGridPositive1DwithStatement[
     $\alpha \mapsto -(\text{JKLinInterval}[\alpha, \text{pI}@\lambda, K] + 10^{-4})$ ,
    Interval[{0.15, 0.45}], 25
  ]
]]

```

Problems: 0 in 0.032062s.

Success on Interval[{0.15, 0.45}]
